# Supplementary material for: Object-Proposal Evaluation Protocol is 'Gameable'
Source: arXiv:1505.05836 source file (2015-11-23)
Supplement: Supplementary file 2 [file supp_AnnotationStatistics.tex]

\paragraph{Statistics of PASCAL vs Non PASCAL annotations}
We noted in the take-away message in section \ref{section:results} of our paper that DMPs were still doing better than other proposals on fully annotated datasets. This is because of the imbalance in the number of PASCAL and non PASCAL annotations. Table \ref{tab:StatisticsTable} summarizes the statistics of annotations on various datasets.

\begin{table*}[!t]
	\centering
	\begin{tabular}{| l |l |l|}
%   \begin{tabular}{|lll|}
    \hline
     & PASCAL Context & MS COCO  \\ \hline 
     non PASCAL classes & 26027 & 129077 \\ \hline
     PASCAL classes & 26691& 167415 \\ \hline
    \end{tabular}
	\captionof{table}{ Annotation statistics of PASCAL and non PASCAL classes} \label{tab:StatisticsTable} 
\end{table*}
