# Supplementary material for: Object-Proposal Evaluation Protocol is 'Gameable'
Source: arXiv:1505.05836 source file (2015-11-23)
Supplement: Supplementary file 3 [file supp_space_saver.tex]

% Some illegal space-saving macros
%\parskip=3pt
\abovedisplayskip 3.0pt plus2pt minus2pt%
\belowdisplayskip \abovedisplayskip

\newlength{\sectionReduceTop}
\newlength{\sectionReduceBot}
\newlength{\subsectionReduceTop}
\newlength{\subsectionReduceBot}
\newlength{\abstractReduceTop}
\newlength{\abstractReduceBot}
\newlength{\captionReduceTop}
\newlength{\captionReduceBot}
%\newlength{\nameReduceTop}
\newlength{\subsubsectionReduceTop}
\newlength{\subsubsectionReduceBot}

\newlength{\eqnReduceTop}
\newlength{\eqnReduceBot}

\newlength{\horSkip}
\newlength{\verSkip}

\newlength{\figureHeight}
\setlength{\figureHeight}{1.7in}

%\newlength{\figureFraction}
\setlength{\horSkip}{-.09in}
\setlength{\verSkip}{-.1in}
\setlength{\subsectionReduceTop}{-0.05in}
\setlength{\subsectionReduceBot}{-0.05in}
\setlength{\sectionReduceTop}{-0.06in}
\setlength{\sectionReduceBot}{-0.06in}
\setlength{\subsubsectionReduceTop}{-0.06in}
\setlength{\subsubsectionReduceBot}{-0.05in}
\setlength{\abstractReduceTop}{-0.05in}
\setlength{\abstractReduceBot}{-0.10in}

\setlength{\eqnReduceTop}{-0.05in}
\setlength{\eqnReduceBot}{-0.05in}

\setlength{\captionReduceTop}{-0.14in}
\setlength{\captionReduceBot}{-0.12in}
